# Supplementary material for: Optimal design of calibration signals in space borne gravitational wave detectors
Source: arXiv:1511.09198 source file (2015-11-30)
Supplement: Supplementary file 1 [file appendix.tex]

\appendix
